# Supplementary material for: Deviations from the Porter-Thomas Distribution due to Nonstatistical $\gamma$ Decay below the $^{150}$Nd Neutron Separation Threshold
Source: arXiv:2501.19185 ancillary file (2025-07-30)
Supplement: Supplementary file 1 [file supplemental.pdf]

# Supplemental Material for "Deviations from the Porter-Thomas distribution due to non-statistical $\gamma$ decay below the $^{150}$Nd neutron separation threshold"

O. Papst [1,*] J. Isaak [1,†] V. Werner [1] D. Savran [2] N. Pietralla [1] G. Battaglia [3] T. Beck [1,‡] M. Beuschlein [1] S. W. Finch [4,5] U. Friman-Gayer [1,§] K. E. Ide [1] R. V. F. Janssens [5,6] M. D. Jones [5,6] J. Kleemann [1] B. Löher [2] M. Scheck [7,8] M. Spieker [9,¶] W. Tornow [4,5] R. Zidarova [1] and A. Zilges [10]

[1] *Technische Universität Darmstadt, Department of Physics, Institute for Nuclear Physics, 64289 Darmstadt, Germany*
[2] *GSI Helmholtzzentrum für Schwerionenforschung GmbH, 64291 Darmstadt, Germany*
[3] *University of Strathclyde, Glasgow G4 0NG, United Kingdom*
[4] *Department of Physics, Duke University, Durham, NC 27708-0308, USA*
[5] *Triangle Universities Nuclear Laboratory, Durham, NC 27708-0308, USA*
[6] *Department of Physics and Astronomy, University of North Carolina at Chapel Hill, Chapel Hill, NC 27599, USA*
[7] *School of Computing, Engineering, and Physical Sciences, University of the West of Scotland, Paisley PA1 2BE, United Kingdom*
[8] *The Scottish Universities Physics Alliance, Glasgow G12 8QQ, United Kingdom*
[9] *National Superconducting Cyclotron Laboratory, Michigan State University, East Lansing, MI 48824, USA*
[10] *Institut für Kernphysik, Universität zu Köln, 50937 Köln, Germany*

## SUPPLEMENTARY MATERIAL

This supplementary material provides additional details and data supporting the results presented in the main text. It includes a derivation of the internal fluctuation ratio used in the analysis, an investigation of contributions arising from non-statistical $\gamma$ decays, and a table listing the experimental results for the photon-scattering cross sections and average branching ratios for each photon beam energy.

### Internal fluctuation ratio

The experimentally observed cross sections depend on the transition widths of the excited states. The partial transition widths of the individual transitions are assumed to fluctuate around the average value according to some distribution $f_i$ and $g_i$:

$$\Gamma_{0,i} = \langle \Gamma_0 \rangle \cdot f_i, \qquad \Gamma_{2,i} = \langle \Gamma_2 \rangle \cdot f_i', \qquad \Gamma_i = \langle \Gamma \rangle \cdot g_i. \quad (1)$$

Inserting these relations into Eq. (2) in the main article yields

$$\frac{\sum_{i=0}^{M} \Gamma_{0,i} \frac{\Gamma_{2,i}}{\Gamma_i}}{\sum_{i=0}^{M} \Gamma_{0,i} \frac{\Gamma_{0,i}}{\Gamma_i}} = \frac{\sum_{i=0}^{M} \langle \Gamma_0 \rangle f_i \cdot \langle \Gamma_2 \rangle f_i' / \langle \Gamma \rangle g_i}{\sum_{i=0}^{M} \langle \Gamma_0 \rangle f_i \cdot \langle \Gamma_0 \rangle f_i / \langle \Gamma \rangle g_i} \quad (2)$$

$$= \frac{\langle \Gamma_2 \rangle}{\langle \Gamma_0 \rangle} \frac{\sum_{i=0}^{M} f_i \cdot f_i' / g_i}{\sum_{i=0}^{M} f_i \cdot f_i / g_i} \equiv \frac{\langle \Gamma_2 \rangle}{\langle \Gamma_0 \rangle} \cdot s. \quad (3)$$

The index $i$ sums over $M$ excited states. Assuming $\chi^2$-distributed partial transition widths, the total transition widths are Gaussian-distributed, i.e.,

$$f_i \sim \chi^2(\nu)/\nu, \qquad f_i' \sim \chi^2(\nu)/\nu, \quad (4)$$

$$g_i \sim \frac{1}{N} \sum_{j=0}^{N} \chi^2(\nu)/\nu \xrightarrow{N \to \infty} \mathcal{N}(\mu = \nu, \sigma^2 = 2\nu/N)/\nu. \quad (5)$$

Here, $N$ refers to the number of partial transition widths contributing to $\Gamma_i$. Thus, the internal fluctuation ratio $s$ only depends on the degree of freedom $\nu$ of the $\chi^2(\nu)$ distribution.

In the following, a generalization of the $\chi^2$ distribution for $\nu \in \mathbb{R}^+$ based on the gamma distribution is used. In its limit definition, $g_i$ is statistically independent of $f_i$ and $f_i'$, which follows directly from the central limit theorem. Using (a) the central limit theorem and (b) the independence of $f_i, f_i'$, and $g_i$ for different $i$, its expectation value $\mathrm{E}[s]$ is calculated as

$$\mathrm{E}[s] \equiv \mathrm{E}\left[\frac{\sum_i f_i \cdot f_i'/g_i}{\sum_i f_i \cdot f_i/g_i}\right] \overset{(a)}{=} \frac{\sum_i \mathrm{E}\left[f_i \cdot f_i'/g_i\right]}{\sum_i \mathrm{E}\left[f_i \cdot f_i/g_i\right]} \quad (6)$$

$$\overset{(b)}{=} \frac{M}{M} \frac{\mathrm{E}\left[f \cdot f'/g\right]}{\mathrm{E}\left[f \cdot f/g\right]} = \frac{\mathrm{E}\left[f \cdot f'/g\right]}{\mathrm{E}\left[f \cdot f/g\right]}. \quad (7)$$

The contribution from $g \sim \mathcal{N}(\mu, \sigma^2)$, which is present in both the expectation value of the numerator and the denominator, is approximately constant, as its variance $\sigma^2 = 2\nu/N$ decreases with increasing number $N$ of transitions to lower-lying states. Instead, the simplified expression

$$\mathrm{E}[s] = \frac{\mathrm{E}\left[f \cdot f'\right]}{\mathrm{E}\left[f \cdot f\right]} \quad (8)$$

is calculated.

The numerator is a product of two independent random variables that can be separated, i.e., $\mathrm{E}\left[f \cdot f'\right] = \mathrm{E}[f] \cdot \mathrm{E}[f'] = \nu^2$, using $\mathrm{E}[f] = \nu$ for the $\chi^2$ distribution. The denominator is the expectation value of the square of a random variable, which is (c) equivalent to its second moment. Given the probability

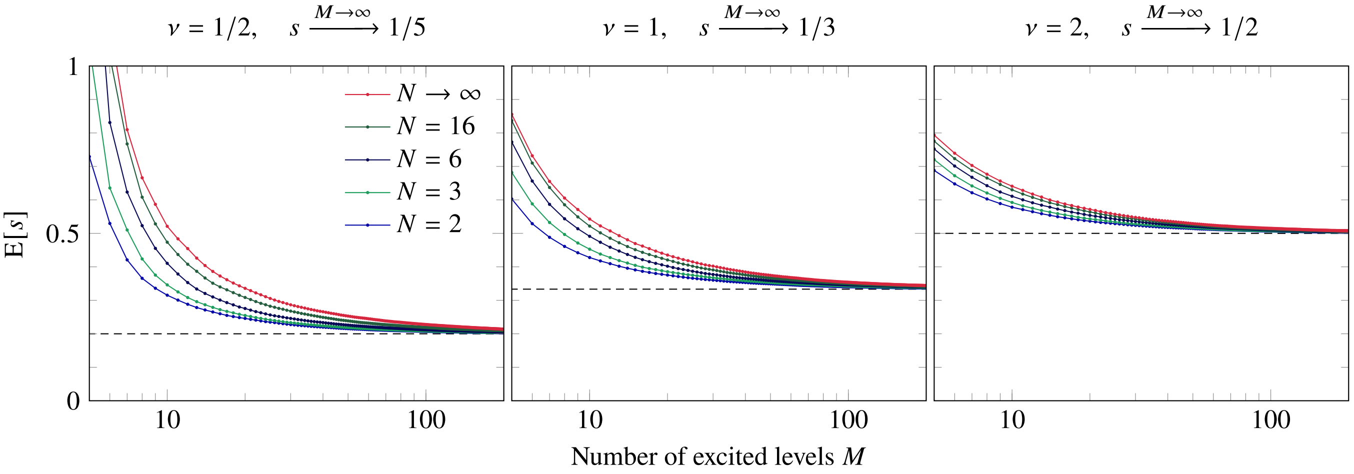


FIG. 1. Convergence of the expectation value $\mathrm{E}[s]$ of the internal fluctuation ratio $s$ as a function of the number of excited levels $M$ and the number of partial transition widths $N$ that contribute to $\langle\Gamma\rangle$. The degree of freedom $\nu$ and the limit of the internal fluctuation ratio $s$ for large $M$ are given above each panel.

density function (PDF) of the $\chi^2(\nu)$ distribution

$$f_{\chi^2}(x \mid \nu) = \frac{1}{2^{\nu/2}\Gamma(\nu/2)} x^{\nu/2-1} \exp(-x/2), \tag{9}$$

with the gamma function $\Gamma(x)$, the expectation value can be calculated using

$$\begin{aligned}
\mathrm{E}[f \cdot f] &\overset{(c)}{=} \int_0^\infty x^2 f_{\chi^2}(x \mid \nu)\,\mathrm{d}x & (10)\\
&\equiv \int_0^\infty x^2 \frac{1}{2^{\nu/2}\Gamma(\nu/2)} x^{\nu/2-1} \exp(-\nu/2)\,\mathrm{d}x & (11)\\
&= \frac{4\Gamma(\nu/2+2)}{\Gamma(\nu/2)} & (12)\\
&\overset{(d)}{=} 2\nu(\nu/2+1) = \nu(\nu+2). & (13)
\end{aligned}$$

For (d), $\Gamma(z+1) = z\Gamma(z)$ is used.

In conclusion,

$$s = \frac{\mathrm{E}[f \cdot f']}{\mathrm{E}[f \cdot f]} = \frac{\nu^2}{\nu(\nu+2)} = \frac{\nu}{\nu+2} \quad \Leftrightarrow \quad \nu = \frac{2s}{1-s}, \tag{14}$$

with the following special cases:

$$s(\nu = 0.5) = 1/5, \quad s(\nu = 1) = 1/3, \quad s(\nu = 2) = 1/2 \tag{15}$$

The convergence of $s$ for different numbers $N$ of partial transition widths and different numbers $M$ of states in the excitation-energy region is illustrated in Fig. 1. The plot was generated by sampling from the individual probability distributions. If fewer transitions and thus partial transition widths $N$ contribute to $\langle\Gamma\rangle$, the convergence is even faster than for the limit of $N \to \infty$. Thus, even if only $\Gamma = \Gamma_0 + \Gamma_2$, the expectation value $\mathrm{E}[s]$ for $s$ converges for sufficiently large numbers of excited levels $M$.

As can be seen in Fig. 1, if the number of excited states $M$ within an energy region is too small, the expectation value $\mathrm{E}[s]$ is larger than its limit for large $M$. For $^{150}$Nd, the internal fluctuation ratio is expected to converge: Both constant temperature (CT) and back-shifted Fermi gas (BSFG) nuclear level density (NLD) models agree that the average level spacing for $1^-$ states is around 2 keV for $E = 5$ MeV ($\rho^{1^-}(5\,\mathrm{MeV}) = 500\,\mathrm{MeV}^{-1}$), and decreases to about 0.1 keV for $E = 7$ MeV ($\rho^{1^-}(7\,\mathrm{MeV}) = 1 \times 10^4\,\mathrm{MeV}^{-1}$). The NLDs observed in Oslo-method experiments for $^{150}$Nd [1] are slightly lower but confirm the order of magnitude. This ensures that $s$ converges. The statistical model simulation depicted in Fig. 2 in the main article also takes into account the NLD such that this effect is already quantified by the simulation and its uncertainties. For higher excitation energies, the NLD increases, and the experimental values should get closer to the limit value for $\mathrm{E}[s]$.

**Contribution from non-statistical $\gamma$ decays**

The measured average branching ratio $\langle R_{\mathrm{exp}}\rangle$ given in Eq. (6) of the main article is separated into three components that account for contributions in the ground-state decay cross section following pure statistical decay and decay properties expected from the Alaga rule [2] for $K = 0$ and $K = 1$ states. In the following, a detailed derivation of Eq. (6) is given.

$$\begin{aligned}
\langle R_{\mathrm{exp}}\rangle &= \frac{\sum_i I_{2,i}}{\sum_i I_{0,i}} \frac{E^3_{\gamma_0}}{E^3_{\gamma_2}} & (16)\\
&= \frac{\left[\sum_j I_{2,j}\right]_{\mathrm{stat}} + \left[\sum_k I_{2,k}\right]_{K=0} + \left[\sum_l I_{2,l}\right]_{K=1}}{\sum_i I_{0,i}} \frac{E^3_{\gamma_0}}{E^3_{\gamma_2}} & (17)
\end{aligned}$$

Equation (16) can be simplified using the following expressions for the three terms in the numerator:

$$\frac{\left[\sum_j I_{2,j}\right]_{\text{stat}}}{\left[\sum_j I_{0,j}\right]_{\text{stat}}} = s\frac{\langle\Gamma_2\rangle}{\langle\Gamma_0\rangle} \tag{18}$$

$$\Rightarrow \left[\sum_j I_{2,j}\right]_{\text{stat}} = s\frac{\langle\Gamma_2\rangle}{\langle\Gamma_0\rangle}\left[\sum_j I_{0,j}\right]_{\text{stat}} \tag{19}$$

$$\left[\sum_k I_{2,k}\right]_{K=0} = 2\frac{E^3_{\gamma_2}}{E^3_{\gamma_0}}\left[\sum_k I_{0,k}\right]_{K=0} \tag{20}$$

$$\left[\sum_l I_{2,l}\right]_{K=1} = 0.5\frac{E^3_{\gamma_2}}{E^3_{\gamma_0}}\left[\sum_l I_{0,l}\right]_{K=1} \tag{21}$$

The relations in Eqs. (20) and (21) are derived according to the Alaga rule [2]

$$\frac{\Gamma_{2,k}}{\Gamma_{0,k}}\frac{E^3_{\gamma_0}}{E^3_{\gamma_2}} = 2 \qquad \text{for } K=0 \text{ states} \tag{22}$$

$$\frac{\Gamma_{2,l}}{\Gamma_{0,l}}\frac{E^3_{\gamma_0}}{E^3_{\gamma_2}} = 0.5 \qquad \text{for } K=1 \text{ states} \tag{23}$$

used in the following steps:

$$\left[\sum_k I_{2,k}\right]_{K=0} \propto \left[\sum_k \Gamma_{0,k}\frac{\Gamma_{2,k}}{\Gamma_k}\right]_{K=0} \tag{24}$$

$$= 2\frac{E^3_{\gamma_2}}{E^3_{\gamma_0}}\left[\sum_k \Gamma_{0,k}\frac{\Gamma_{0,k}}{\Gamma_k}\right]_{K=0} \tag{25}$$

$$\propto 2\frac{E^3_{\gamma_2}}{E^3_{\gamma_0}}\left[\sum_k I_{0,k}\right]_{K=0} \tag{26}$$

$$\left[\sum_l I_{2,l}\right]_{K=1} \propto \left[\sum_l \Gamma_{0,l}\frac{\Gamma_{2,l}}{\Gamma_l}\right]_{K=1} \tag{27}$$

$$= 0.5\frac{E^3_{\gamma_2}}{E^3_{\gamma_0}}\left[\sum_l \Gamma_{0,l}\frac{\Gamma_{0,l}}{\Gamma_l}\right]_{K=1} \tag{28}$$

$$\propto 0.5\frac{E^3_{\gamma_2}}{E^3_{\gamma_0}}\left[\sum_l I_{0,l}\right]_{K=1} \tag{29}$$

As a result, Eq. (16) is rewritten to

$$\langle R_{\text{exp}}\rangle = s\frac{\langle\Gamma_2\rangle}{\langle\Gamma_0\rangle}\frac{E^3_{\gamma_0}}{E^3_{\gamma_2}}C_{\text{stat}} + 2C_{K=0} + 0.5C_{K=1} \tag{30}$$

$$= s\frac{f_{E1}(E_{\gamma_2})}{f_{E1}(E_{\gamma_0})}C_{\text{stat}} + 2C_{K=0} + 0.5C_{K=1} \tag{31}$$

$$= s\frac{f_{E1}(E_{\gamma_2})}{f_{E1}(E_{\gamma_0})}(1 - C_{K=0} - C_{K=1}) \tag{32}$$

$$+ 2C_{K=0} + 0.5C_{K=1}$$

with

$$C_{\text{stat}} = \frac{\left[\sum_j I_{0,j}\right]_{\text{stat}}}{\sum_i I_{0,i}} \tag{33}$$

$$C_{K=0} = \frac{\left[\sum_k I_{0,k}\right]_{K=0}}{\sum_i I_{0,i}} \tag{34}$$

$$C_{K=1} = \frac{\left[\sum_l I_{0,l}\right]_{K=1}}{\sum_i I_{0,i}} \tag{35}$$

$$1 = C_{\text{stat}} + C_{K=0} + C_{K=1} \tag{36}$$

$$f_{E1}(E_{\gamma_i}) = \frac{\langle\Gamma_i\rangle\,\rho(E_x)}{E^3_{\gamma_i}} \tag{37}$$

where $\rho(E_x)$ is the NLD at the excitation energy $E_x$ [3, 4]. Since the $\gamma$ decays compared in the respective ratios always originate from the same beam-energy setting, i.e. same excitation energy, the NLD cancels out.

### Experimental results on photon-scattering cross sections and average branching ratios

This document contains the tabulated experimental data presented in the associated article. The table is also available as a plain text file (csv format).

In addition to the results discussed in the main article, the table lists the experimentally observed asymmetry $\langle\varepsilon\rangle$ between $E1$ and $M1$ radiation (which is corrected for any effects related to the finite detector size and efficiency), i.e.,

$$\langle\varepsilon\rangle = \frac{\left\langle\frac{\Gamma_0\Gamma_0}{\Gamma}\right\rangle^{M1} - \left\langle\frac{\Gamma_0\Gamma_0}{\Gamma}\right\rangle^{E1}}{\left\langle\frac{\Gamma_0\Gamma_0}{\Gamma}\right\rangle^{M1} + \left\langle\frac{\Gamma_0\Gamma_0}{\Gamma}\right\rangle^{E1}}. \tag{38}$$

TABLE I: Photon-scattering cross sections for each $\gamma$-ray beam energy setting $E_{\text{beam}}$. FWHM gives the full-width at half maximum of the energy distribution of the $\gamma$-ray beam. The photoscattering cross section $\sigma_{\gamma\gamma}$ only corresponds to ground-state decays and is also given as a decomposition into $E1$ and $M1$ contributions. The $M1$ strength contributes only little at higher excitation energies, and its values are expected to be in the order of magnitude of systematic uncertainties. $\langle\varepsilon\rangle$ corresponds to the asymmetry between $M1$ and $E1$ strength.

| $E_{\text{beam}}$ (MeV) | FWHM (keV) | $\sigma_{\gamma\gamma}$ (mb) | $\sigma_{\gamma\gamma}^{E1}$ (mb) | $\sigma_{\gamma\gamma}^{M1}$ (mb) | $\langle R_{\text{exp}}\rangle$ | $\langle R_{\text{exp}}^{M1}\rangle$ * | $\langle\varepsilon\rangle$ |
|---|---|---|---|---|---|---|---|
| 2.95 | 100 | 0.66(6) | 0.088(17) | 0.57(4) | $1.3^{+0.6}_{-1.0}$ | <0.73 | 0.732(32) |
| 3.11 | 109 | 0.46(5) | 0.030(14) | 0.433(34) | $5.2^{+2.4}_{-3.3}$ | <0.42 | 0.87(5) |
| 3.22 | 87 | 0.306(32) | 0.068(15) | 0.238(19) | 1.1(5) | <0.40 | 0.56(5) |
| 3.31 | 109 | 0.271(30) | 0.064(16) | 0.207(18) | 0.6(4) | <0.30 | 0.53(7) |
| 3.41 | 112 | 0.209(26) | 0.075(16) | 0.133(12) | $0.4^{+0.2}_{-0.4}$ | <0.63 | 0.28(8) |
| 3.52 | 115 | 0.194(25) | 0.080(16) | 0.114(11) | 2.0(4) | <0.67 | 0.18(8) |
| 3.62 | 116 | 0.42(4) | 0.310(33) | 0.113(11) | $0.56^{+0.11}_{-0.08}$ | <0.89 | −0.464(35) |
| 3.71 | 119 | 0.56(5) | 0.35(4) | 0.205(17) | $1.10^{+0.11}_{-0.08}$ | <0.50 | −0.263(31) |
| 3.81 | 124 | 0.254(29) | 0.078(17) | 0.176(16) | 1.2(7) | <0.98 | 0.38(7) |
| 3.90 | 128 | 0.31(3) | 0.165(24) | 0.142(14) | $0.10^{+0.05}_{-0.10}$ | <0.32 | −0.07(6) |
| 4.02 | 102 | 0.41(4) | 0.32(3) | 0.090(9) | $0.81^{+0.16}_{-0.10}$ | <1.62 | −0.557(30) |
| 4.10 | 106 | 0.39(4) | 0.254(29) | 0.137(12) | 1.34(11) | <0.65 | −0.30(4) |
| 4.22 | 104 | 0.311(33) | 0.225(27) | 0.085(8) | 0.69(9) | <0.76 | −0.45(4) |
| 4.31 | 108 | 0.33(4) | 0.244(29) | 0.089(9) | 0.64(6) | <0.43 | −0.46(4) |
| 4.39 | 110 | 0.325(34) | 0.150(22) | 0.174(16) | 0.66(8) | <0.15 | 0.08(6) |
| 4.50 | 114 | 0.285(32) | 0.216(27) | 0.069(8) | 0.65(15) | <1.67 | −0.52(4) |
| 4.60 | 109 | 0.35(4) | $0.30^{+0.03}_{-0.04}$ | 0.052(6) | 0.59(7) | <1.20 | $-0.704^{+0.024}_{-0.031}$ |
| 4.70 | 113 | 0.31(3) | 0.237(28) | 0.070(7) | 0.78(6) | <0.46 | −0.54(4) |
| 4.79 | 122 | 0.293(32) | 0.235(27) | 0.058(6) | 0.94(8) | <0.77 | −0.60(3) |
| 4.89 | 117 | 0.36(4) | 0.11(10) | 0.23(16) | $0.9^{+2.5}_{-0.9}$ | <5.04 | 0.3(6) |
| 5.00 | 100 | 0.40(4) | 0.34(4) | 0.056(7) | 0.59(5) | <0.90 | −0.718(28) |
| 5.10 | 98 | 0.42(4) | 0.37(4) | 0.055(7) | 0.75(4) | <0.75 | −0.735(25) |
| 5.21 | 103 | 0.54(5) | 0.49(5) | 0.045(6) | 0.468(32) | <1.02 | −0.831(20) |
| 5.31 | 109 | 0.52(5) | 0.47(5) | 0.049(6) | 0.484(31) | <0.97 | −0.810(19) |
| 5.40 | 104 | 0.59(6) | 0.54(5) | 0.050(7) | 0.597(29) | <0.87 | −0.830(19) |
| 5.51 | 106 | 0.90(8) | 0.85(7) | 0.046(7) | $0.396^{+0.027}_{-0.021}$ | <1.52 | −0.897(15) |
| 5.61 | 109 | 0.71(6) | 0.66(6) | 0.052(7) | 0.605(25) | <0.67 | −0.852(17) |
| 5.71 | 115 | 0.76(7) | 0.72(7) | 0.038(7) | $0.519^{+0.029}_{-0.019}$ | <1.13 | −0.899(16) |
| 5.78 | 125 | 0.89(8) | 0.83(7) | 0.053(7) | 0.432(16) | <0.50 | $-0.881^{+0.015}_{-0.011}$ |
| 5.81 | 120 | 0.99(8) | 0.94(8) | 0.044(9) | $0.316^{+0.023}_{-0.017}$ | <1.26 | −0.910(17) |
| 5.91 | 120 | 0.81(7) | 0.76(7) | 0.053(7) | 0.564(22) | <0.69 | −0.869(16) |
| 6.02 | 109 | 0.98(8) | 0.92(8) | 0.061(9) | 0.424(22) | <1.01 | −0.876(16) |
| 6.06 | 154 | 1.13(10) | 1.05(9) | 0.082(11) | 0.366(19) | <0.58 | −0.855(17) |

Continued on next page

TABLE I: (Continued)

| $E_{beam}$ (MeV) | FWHM (keV) | $\sigma_{\gamma\gamma}$ (mb) | $\sigma_{\gamma\gamma}^{E1}$ (mb) | $\sigma_{\gamma\gamma}^{M1}$ (mb) | $\langle R_{exp} \rangle$ | $\langle R_{exp}^{M1} \rangle$ * | $\langle \varepsilon \rangle$ |
|---|---|---|---|---|---|---|---|
| 6.12 | 115 | 0.93(8) | 0.85(7) | 0.078(9) | 0.459(20) | <0.46 | −0.832(16) |
| 6.20 | 118 | 0.77(7) | 0.70(6) | 0.069(8) | 0.519(21) | <0.37 | $-0.818^{+0.019}_{-0.014}$ |
| 6.30 | 121 | 0.74(7) | 0.69(6) | 0.054(7) | 0.486(23) | <0.70 | −0.853(17) |
| 6.40 | 117 | 0.56(5) | 0.50(5) | 0.064(7) | 0.688(31) | <0.34 | −0.772(21) |
| 6.50 | 114 | 0.65(6) | 0.61(6) | 0.045(7) | 0.471(26) | <0.72 | −0.862(20) |
| 6.59 | 128 | 0.66(6) | 0.60(6) | 0.058(8) | $0.502^{+0.027}_{-0.022}$ | <0.49 | −0.824(20) |
| 6.69 | 141 | 0.52(5) | 0.48(5) | 0.042(6) | 0.602(32) | <0.52 | −0.840(22) |
| 6.79 | 134 | 0.54(5) | 0.47(5) | 0.065(8) | 0.543(31) | <0.47 | −0.759(22) |
| 6.89 | 130 | 0.57(6) | 0.45(5) | 0.11(4) | 0.44(4) | <0.33 | −0.60(11) |
| 6.99 | 131 | 0.45(4) | 0.39(4) | 0.057(9) | 0.63(5) | <0.96 | −0.74(4) |

* Given as $2\sigma$ upper limits.


* opapst@ikp.tu-darmstadt.de
† jisaak@ikp.tu-darmstadt.de
‡ Present address: KU Leuven, Instituut voor Kern- en Stralingsfysica, 3001 Leuven, Belgium
§ Present address: Vysus Group Sweden AB, 214 21 Malmö, Sweden
¶ Present address: Department of Physics, Florida State University, Tallahassee, FL 32306, USA



[1] M. Guttormsen *et al.*, Phys. Lett. B **816**, 136206 (2021).
[2] G. Alaga, K. Alder, A. Bohr, and B. R. Mottelson, Dan. Mat. Fys. Medd. **29** (1955).
[3] G. A. Bartholomew, E. D. Earle, A. J. Ferguson, J. W. Knowles, and M. A. Lone, Gamma-ray strength functions, in *Advances in Nuclear Physics*, Vol. 7, edited by M. Baranger and E. Vogt (Springer Science and Business Media LLC, New York, NY, USA, 1973) Chap. 4, pp. 229–324.
[4] S. Goriely, P. Dimitriou, M. Wiedeking, T. Belgya, R. Firestone, J. Kopecky, M. Krtička, V. Plujko, R. Schwengner, S. Siem, H. Utsunomiya, S. Hilaire, S. Péru, Y. S. Cho, D. M. Filipescu, N. Iwamoto, T. Kawano, V. Varlamov, and R. Xu, Eur. Phys. J. A **55**, 172 (2019).
